# Supplementary material for: CompilerGym: Robust, Performant Compiler Optimization Environments for AI Research
Source: arXiv:2109.08267 source file (2021-12-22)
Supplement: Supplementary file 1 [file artifact-evaluation.tex]

\section{Artifact Appendix}

\lstset{%
    frame=l,
    rulecolor=\color{red},
}

\subsection{Abstract}

Our artifact comprises source code and pre-compiled binaries for CompilerGym,
and instructions to reproduce the nine experiments in the paper.

\subsection{Artifact check-list (meta-information)}

{\small
\begin{itemize}
  \item {\bf Run-time environment: } Ubuntu 18.04, Fedora 28, Debian 10 or
  newer, or macOS. Python 3.8.
  \item {\bf Experiments: } Computational efficiency benchmarks; autotuning for
  LLVM phase ordering, GCC command line flags, and CUDA loop nests; supervised
  graph learning; and reinforcement learning for LLVM phase ordering.
  \item {\bf How much disk space required (approximately)?: } 20GB.
  \item {\bf How much time is needed to prepare workflow (approximately)?: } 15
  minutes.
  \item {\bf How much time is needed to complete experiments (approximately)?: }
  3 hours.
  \item {\bf Publicly available?: } Yes. \url{https://compilergym.ai}
\end{itemize}
}

\subsection{Description}

\subsubsection{How delivered}

The artifact is available from:\\*
\url{https://doi.org/10.5281/zenodo.5784251}.

\subsubsection{Hardware dependencies}

We recommend a minimum of 64GB RAM. We used a commodity desktop machine equipped
with a AMD Ryzen 9 3900X CPU and NVIDIA 2080 GPU to generate the compute time
estimates in this document.
A CUDA-equipped GPU is required for one of the experiments
(Section~\ref{subsection:autotuning-loop-tool}).
The following experiments contain runtime measurements and so will produce
different vakyes on your system:
Sections~\ref{subsection:computational-efficiency},
\ref{subsection:observation-spaces-efficiency},
\ref{subsection:autotuning-llvm}, and~\ref{subsection:autotuning-loop-tool}. The
remainder of the experiments are hardware-agnostic.

\subsubsection{Software dependencies}

All experiments require Python 3.8. We recommend using anaconda to prevent
interference with your system Python.
Docker is required for one of the experiments
(Section~\ref{subsection:autotuning-gcc}).

\subsection{Installation}

(Optional) Use conda\footnote{If not already available, see the documentation
for installation
instructions:\\*\url{https://docs.conda.io/projects/conda/en/latest/user-guide/install/index.html}}
to create a clean Python environment:
\begin{lstlisting}
conda create -y -n compiler_gym python=3.8
conda activate compiler_gym
\end{lstlisting}
\noindent
Confirm that your environment is using Python 3.8:
\begin{lstlisting}
python --version
\end{lstlisting}
\noindent
Next, install the \cg{} library using:
\begin{lstlisting}
python -m pip install -U compiler_gym
\end{lstlisting}
\noindent
Either download the artifact archive linked above, or clone the repository to
get the most recent version using:
\begin{lstlisting}
git clone \
    https://github.com/facebookresearch/CompilerGym.git
\end{lstlisting}
\noindent
Change to the examples directory and install the dependencies using:
\begin{lstlisting}
cd CompilerGym/examples
python setup.py install
\end{lstlisting}
\noindent
The remainder of this document requires that the user remains in the
\texttt{\scriptsize CompilerGym/examples} directory.

\subsection{Experiments}

This section describes how to reproduce all of the experiments in the paper. The
workflow, evaluation, and customization steps of each experiment is described in
turn.

\vspace{1em}
\noindent
\textbf{(Optional) Getting Started with CompilerGym}

Before running the experiments below we recommend navigating to
\url{https://compilergym.ai/getting_started} and clicking the ``Open in Colab''
button to launch an interactive webpage that describes the main CompilerGym
concepts and APIs. It takes approximately 20 minutes to complete.

\vspace{1em}
\noindent
\textbf{Sections~\ref{subsection:computational-efficiency}
and~\ref{subsection:observation-spaces-efficiency}: Computational Efficiency}

\emph{Workflow:} The following script benchmarks the computation times of the
three environment operations (startup, initialization, and step), and each of
the eight observation spaces:
\begin{lstlisting}
python -m op_benchmarks run --n=200
\end{lstlisting}
\noindent
where \texttt{\footnotesize --n} is the number of runtimes to collect for each
type of operation. Collecting \texttt{\footnotesize --n=200} measurements will
take about 10 minutes. In the paper we use \texttt{\footnotesize --n=1000000}.

\emph{Evaluation:} Aggregate measurements and compare the runtimes to
Table~\ref{table:llvm-op-costs} and Table~\ref{table:llvm-observation-spaces}
using:
\begin{lstlisting}
python -m op_benchmarks info
\end{lstlisting}

\vspace{1em}
\noindent
\textbf{Section~\ref{subsection:autotuning-llvm}: Autotuning LLVM Phase
Ordering}

\emph{Workflow:} Run a single autotuning experiment using:
\begin{lstlisting}
export AUTOTUNER=nevergrad; TARGET=codesize; \
python -m llvm_autotuning.tune -m \
    experiment="${AUTOTUNER}-${TARGET}" \
    autotuner="${AUTOTUNER}" \
    autotuner.optimization_target="${TARGET}" \
    num_replicas=1 \
    autotuner.search_time_seconds=300
\end{lstlisting}
where \texttt{\scriptsize AUTOTUNER} is set to one of \texttt{\scriptsize
nevergrad}, \texttt{\scriptsize random}, \texttt{\scriptsize greedy}, or
\texttt{\scriptsize opentuner}; and \texttt{\scriptsize TARGET} is set to one of
\texttt{\scriptsize codesize}, \texttt{\scriptsize binsize}, or
\texttt{\scriptsize runtime}. Run all 12 combinations of autotuner and target to
reproduce the full suite of experiments in
Section~\ref{subsection:autotuning-llvm}.

The above command will take about 6 minutes to complete. Compared to the
experiment in the paper each autotuner is run only once and with a search budget
of 5 minutes instead of one hour. To replicate the full experiment from
Section~\ref{subsection:autotuning-llvm}, taking about 12 hours, run:
\begin{lstlisting}
export AUTOTUNER=nevergrad; TARGET=codesize; \
python -m llvm_autotuning.tune -m \
    experiment="${AUTOTUNER}-${TARGET}" \
    autotuner="${AUTOTUNER}" \
    autotuner.optimization_target="${TARGET}" \
    num_replicas=10 \
    autotuner.search_time_seconds=3600
\end{lstlisting}

\emph{Evaluation:} Aggregate and compare to Table~\ref{table:llvm-autotuning}
using:
\begin{lstlisting}
python -m llvm_autotuning.info
\end{lstlisting}

\emph{Customization:} The experiment is configurable through several command
line arguments described in \texttt{\scriptsize llvm\_autotuning/README.md}.
Example customizations include \texttt{\scriptsize
autotuner.search\_time\_seconds} to change the search budget, and
\texttt{\scriptsize autotuner.algorithm\_config.episode\_length} to set the
number of steps in Nevergrad environment episodes.

\vspace{1em}
\noindent
\textbf{Section~\ref{subsection:autotuning-gcc}: Autotuning GCC Command Line
Flags}

\emph{Workflow:} Run a small-scale autotuning experiment using:
\begin{lstlisting}
python -m gcc_autotuning.tune \
    --gcc_search_budget=100 \
    --pop_size=20 \
    --gcc_search_repetitions=1 \
    --gcc_benchmark=benchmark://chstone-v0/aes,benchmark://chstone-v0/blowfish,benchmark://chstone-v0/dfmul,benchmark://chstone-v0/dfsin,benchmark://chstone-v0/sha
\end{lstlisting}
\noindent
Note the final \texttt{\footnotesize --gcc\_benchmark} argument above should
entered as a single line without spaces. This requires docker. If docker is not
installed, use \texttt{\footnotesize --gcc\_bin=/path/to/gcc} to specify the
path to a GCC installation. The above command takes about 12 minutes to complete
and uses fewer benchmarks and a smaller search budget than in the paper. To
replicate the full suite setup from Section~\ref{subsection:autotuning-gcc},
taking about 6 hours, run:
\begin{lstlisting}
python -m gcc_autotuning.tune
\end{lstlisting}

\emph{Evaluation:} Aggregate and compare to Table~\ref{table:gcc-autotuning}
using:
\begin{lstlisting}
python -m gcc_autotuning.info
\end{lstlisting}

\emph{Customization:} The experiment is configurable through a number of command
line arguments described in \texttt{\scriptsize gcc\_autotuning/README.md}.
Example customizations include \texttt{\scriptsize --gcc\_search\_budget} to
change the search budget, \texttt{\scriptsize --gcc\_bin} to use a different GCC
binary, and \texttt{\scriptsize --gcc\_benchmark} to change the list of programs
used.

\vspace{1em}
\noindent
\textbf{Section~\ref{subsection:autotuning-loop-tool}: Autotuning CUDA Loop
Nests}

\emph{Workflow:} Run a sweep on a CUDA-capable GPU using:
\begin{lstlisting}
python -m loop_tool_sweep --device=cuda --k=128
\end{lstlisting}
\noindent
This will take approximately 3 minutes to complete. In
Section~\ref{subsection:autotuning-loop-tool} this experiment is repeated using
the following values for \texttt{\scriptsize --k}: 512, 1024, 2048, 4096, and
8192.

\emph{Evaluation:} Compare values logged to stdout to
Figure~\ref{figure:loop-tool-sweep}.

\emph{Customization:} Use \texttt{\scriptsize --k} and \texttt{\scriptsize
--vectorize} to specify the dataset and vectorization sizes, respectively, and
\texttt{\scriptsize --device=cpu} to run on CPU.

\vspace{1em}
\noindent
\textbf{Section~\ref{subsection:sl-offline-dataset}: Learning a Cost Model}

\emph{Workflow:} Train a graph neural network cost model using:
\begin{lstlisting}
python -m gnn_cost_model.train \
    --device=cpu --batch_size=4 \
    --num_epoch=10 --dataset_size=100
\end{lstlisting}
\noindent
The above command takes around 10 minutes to complete and uses 100 graphs from a
small 3 GB state transition dataset. To replicate the full scale experiment of
Section~\ref{subsection:sl-offline-dataset}, run:
\begin{lstlisting}
python -m gnn_cost_model.train --num_epoch=35 \
    --db=https://dl.fbaipublicfiles.com/compiler_gym/state_transition_dataset/2021-11-15-cbench.tar.bz2
    --db_sha256=36dddceca405126a1249c640cba5b678d4a1db3d9298ad7e5f1d
        a2fa4eccfd20
\end{lstlisting}
\noindent
This requires a minimum of 60 GB of RAM and disk space.

\emph{Evaluation:} Compare loss logged to stdout to
Figure~\ref{figure:supervised-learning}.

\emph{Customization:} The training script can be configured through several
command line arguments. List them using:
\begin{lstlisting}
python -m gnn_cost_model.train --help
\end{lstlisting}

\vspace{1em}
\noindent
\textbf{Sections~\ref{subsection:rl-algos}, \ref{subsection:rl-training-set},
and~\ref{subsection:rl-observation-spaces}: Reinforcement Learning}

\emph{Workflow:} Train a PPO~\cite{ppo} agent for 1000 episodes using:

\begin{lstlisting}
python -m llvm_rl.train -m \
    experiment=algo \
    agent=ppo \
    num_replicas=1 \
    training.episodes=1000
\end{lstlisting}
\noindent
This will take approximately 20 minutes to complete. In the paper, agents are
trained for \texttt{\footnotesize training.episodes=100000} and repeated 10
times (\texttt{\footnotesize num\_replicas=10}).

To train using four different algorithms and evaluating on all test sets
(Section~\ref{subsection:rl-algos}), run:
\begin{lstlisting}
python -m llvm_rl.train -m \
    experiment=algo \
    agent=a2c,apex,impala,ppo testing=all
\end{lstlisting}
\noindent
To cross-validate the effect of different training and test sets
(Section~\ref{subsection:rl-training-set}), run:
\begin{lstlisting}
python -m llvm_rl.train -m \
    experiment=training-set \
    training=csmith,github,tensorflow \
    testing=csmith-github-tensorflow
\end{lstlisting}
\noindent
To evaluate the effect of different observation spaces on agents
(Section~\ref{subsection:rl-observation-spaces}), run:
\begin{lstlisting}
python -m llvm_rl.train -m \
    experiment=observation-spaces \
    training.episodes=100000 \
    environment="autophase,autophase-with-history, \
        instcount,instcount-with-history"
\end{lstlisting}

\emph{Evaluation:} Run the following command to provide an overview of the
training progress of each of the agents:
\begin{lstlisting}
python -m llvm_rl.info train
\end{lstlisting}
\noindent
This will print the training time and geometric mean rewards achieved on the
training and validation sets. To summarize agent performance on the holdout test
set(s), run:
\begin{lstlisting}
python -m llvm_rl.info test
\end{lstlisting}

\emph{Customization:} There are a large number of configuration options
available for the experiment, configured through command line arguments. These
are described in \texttt{\scriptsize lvm\_rl/README.md}. Example customizations
include \texttt{\scriptsize agent.type} to specify the reinforcement learning
algorithm to use, \texttt{\scriptsize environment.max\_episode\_steps} to fix
the number of steps in each episode, \texttt{\scriptsize
environment.reward\_space} to specify the objective function to optimize for,
and \texttt{\scriptsize training.episodes} to specify the number of episodes to
train for.

\subsection{Uninstallation}

After completing the evaluation of this artifact, you can delete the conda
environment using:
\begin{lstlisting}
conda deactivate
conda remove --all --name compiler_gym
\end{lstlisting}
\noindent
This will remove the Python package and any installed dependencies. The
following directories can be removed to tidy up CompilerGym's runtime files and
experimental results:
\begin{lstlisting}
rm -rf ~/logs/compiler_gym
rm -rf ~/.local/share/compiler_gym
rm -rf ~/.cache/compiler_gym
\end{lstlisting}

\noindent
Finally, you can delete the directory where you cloned the artifact repository.
