# Supplementary material for: CompilerGym: Robust, Performant Compiler Optimization Environments for AI Research
Source: arXiv:2109.08267 source file (2021-12-22)
Supplement: Supplementary file 2 [file op_costs.tex]

\section{Computational Cost Measurements Further Details}

1M of each operation divided evenly across 1000 benchmarks from each of the 14
datasets. If the dataset has fewer than 1000 benchmarks then they are repeated
to make 1000. Else they were sampled randomly without replacement. For step
measurements, a single episode was used per benchmark, yielding an episode of
length 72 ($\lceil{}\frac{1e^6}{14\times1000}\rceil{}$).

\begin{figure*}
  \centering %
  \includegraphics[width=.95\linewidth]{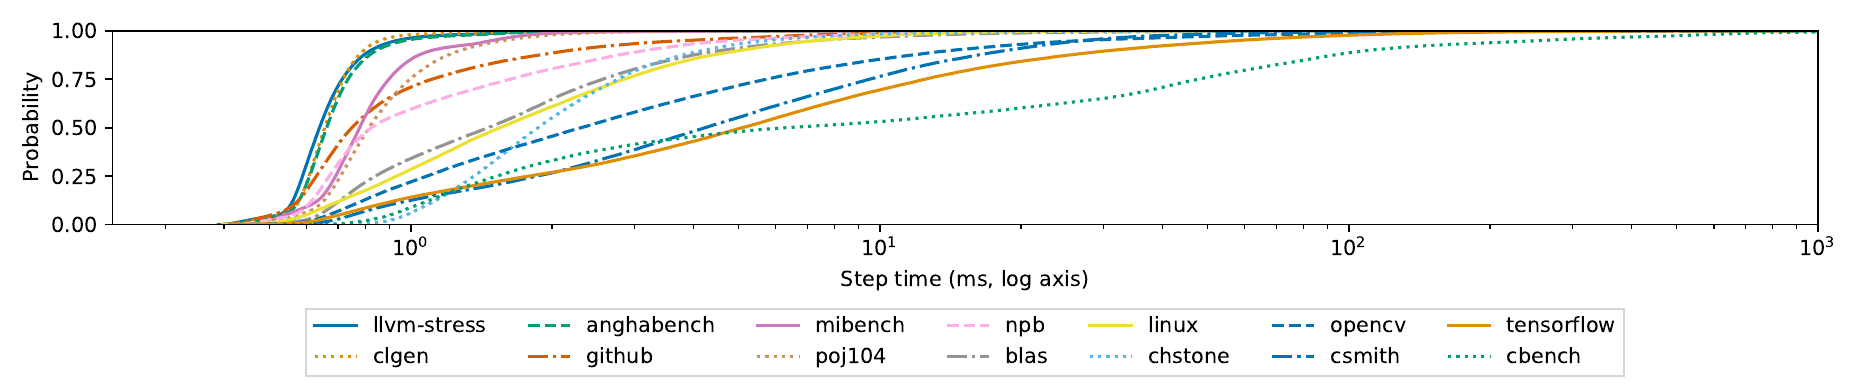}
  \vspace{-1em}
  \caption{%
    Cumulative density plot of step times for datasets, ordered by median step
    time. The difference between the median step of the fastest dataset
    (llvm-stress) and the slowest dataset (cbench) is $9.9\times$.%
  }%
  \label{figure:step-time-cdf-datasets-large}
\end{figure*}

\begin{figure*}
  \centering %
  \includegraphics[width=.95\linewidth]{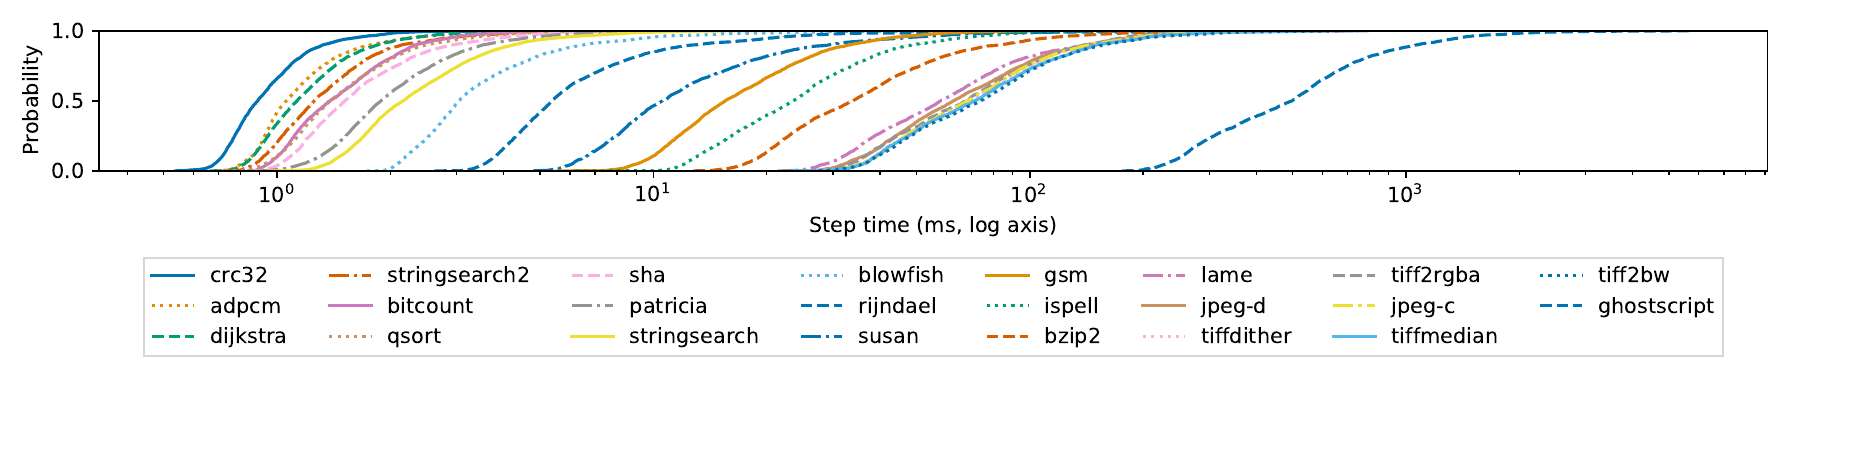}
  \vspace{-3em}
  \caption{%
    Cumulative density plot of step times for each of the 23 programs in
    cBench~\cite{cbench}, ordered by median step time. Wall times measured from
    1M random trials. The difference between the median step times of the
    fastest program (crc32) and the slowest program (ghostbench) is
    560.3$\times$.%
  }%
  \label{figure:step-time-cdf-cbench-large}
\end{figure*}
