# Supplementary material for: CompilerGym: Robust, Performant Compiler Optimization Environments for AI Research
Source: arXiv:2109.08267 source file (2021-12-22)
Supplement: Supplementary file 3 [file search.tex]

\section{Autotuning Experiments Further Details}

We selected the hyperparameters for each autotuning technique through grid search on a holdout set of 100 Csmith programs.

\subsection{Nevergrad}
% Raw data: https://colab.research.google.com/drive/1fs9v1fXc9WB7_Llb8XA-eyvwxsiqs6S_?usp=sharing

We considered 16 optimizers and four fixed episode lengths: 5, 25, 50, 100

\begin{figure*}
  \centering %
  \includegraphics[width=.99\linewidth]{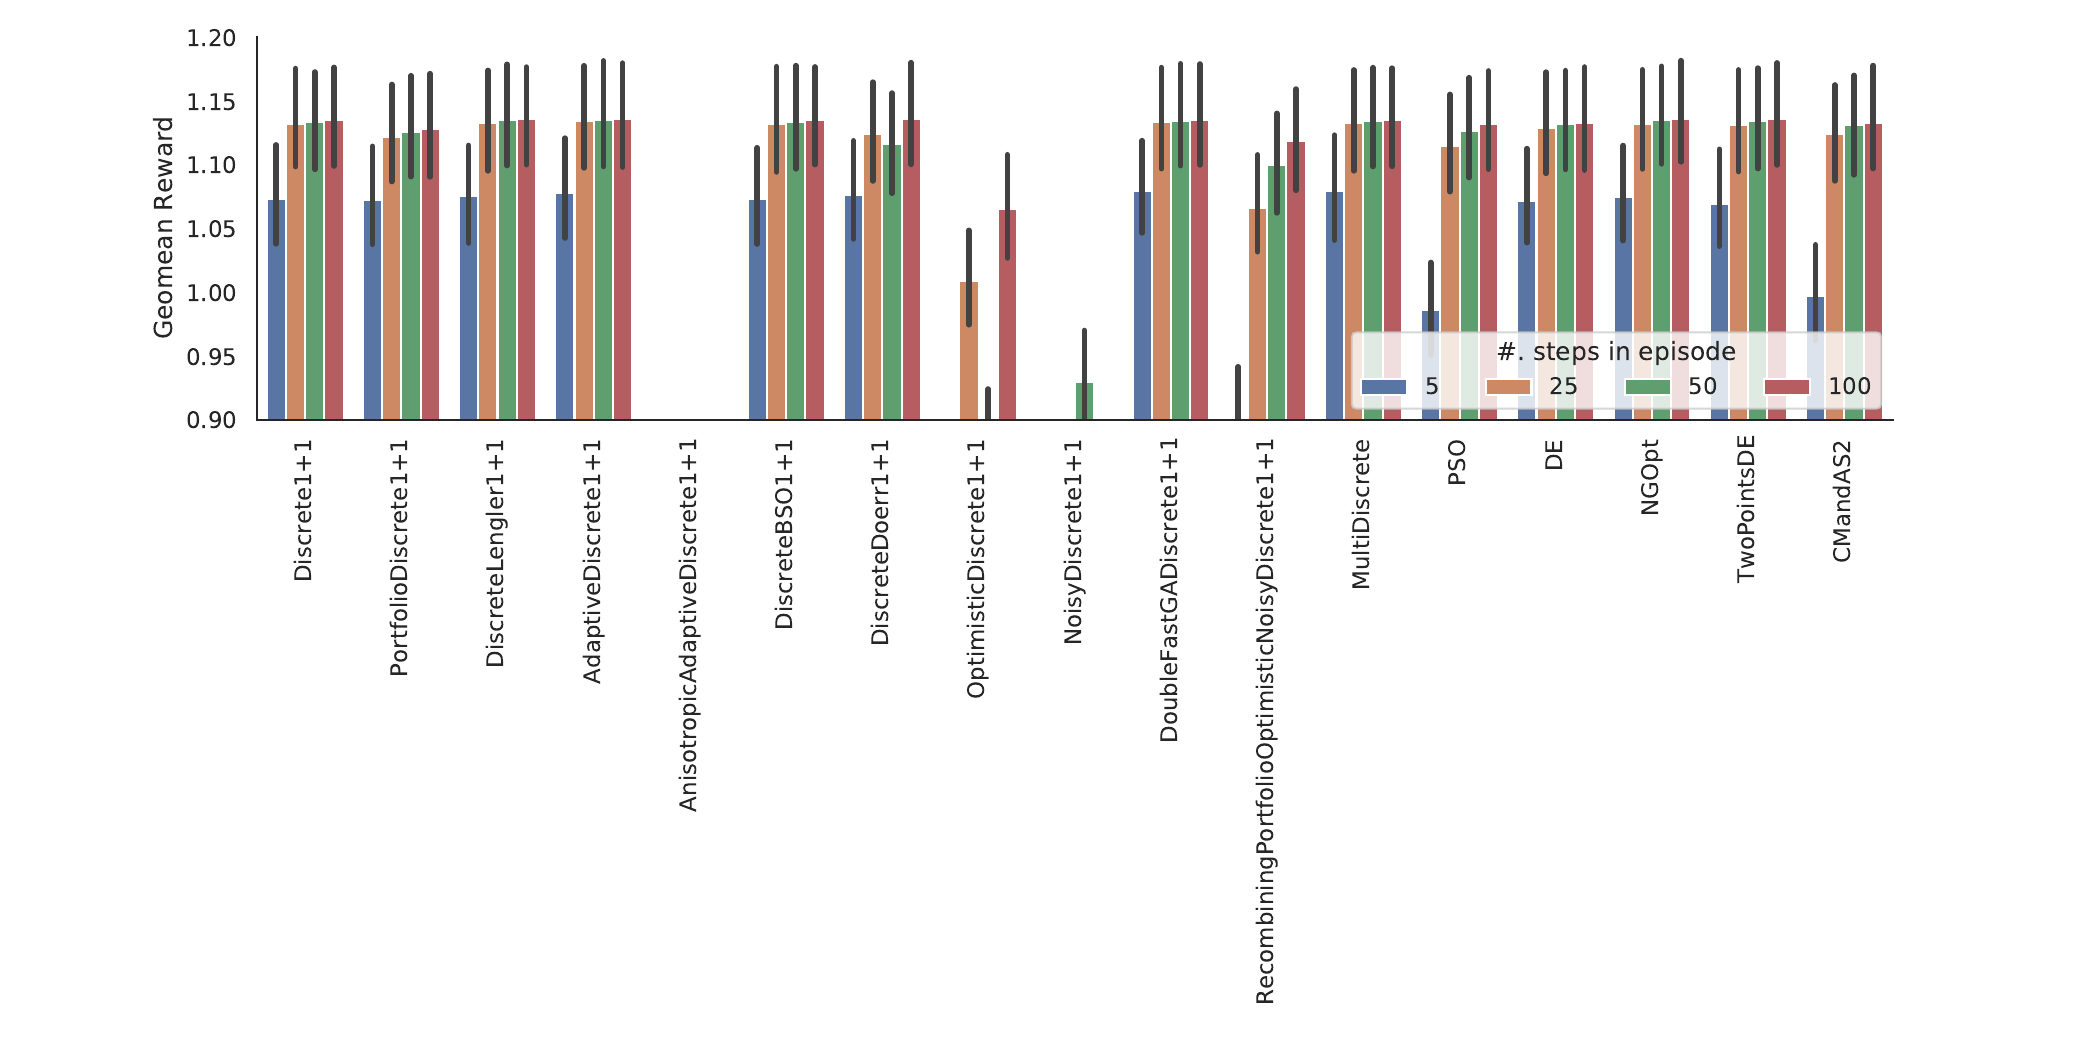}
  \caption{%
    Hyperparameter sweep of black box optimizers using Nevergrad~\cite{nevergrad}. Error bars show 95\% confidence interval.%
  }%
  \label{figure:nevergrad-grid-search}%
\end{figure*}
