# Supplementary material for: CompilerGym: Robust, Performant Compiler Optimization Environments for AI Research
Source: arXiv:2109.08267 source file (2021-12-22)
Supplement: Supplementary file 4 [file supplementary_material.tex]

\title{Deep Data Flow: Appendices}

\maketitle

\appendix
\input{appendix/dataflow_problems}
\input{appendix/dataset}
\input{appendix/experimental_setup}
\input{appendix/downstream_tasks}

\bibliography{refs}
\bibliographystyle{iclr2021_conference}
